# Supplementary material for: Label Efficient Semi-Supervised Learning via Graph Filtering
Source: arXiv:1901.09993 source file (2019-06-28)
Supplement: Supplementary file 1 [file Appendices.tex]

\documentclass[10pt,twocolumn,letterpaper]{article}

\usepackage{times}
\usepackage{epsfig}
\usepackage{amsmath}
\usepackage{amssymb}
\usepackage{amsthm}
\usepackage{amsfonts}       % blackboard math symbols
\usepackage{bm}

\usepackage{graphicx}
\usepackage{caption}
\usepackage{color}
\usepackage[labelformat=simple]{subcaption}

\usepackage{booktabs}       % professional-quality tables
\usepackage[flushleft]{threeparttable}
\usepackage[page,title]{appendix}

% Include other packages here, before hyperref.

% If you comment hyperref and then uncomment it, you should delete
% egpaper.aux before re-running latex.  (Or just hit 'q' on the first latex
% run, let it finish, and you should be clear).
\usepackage[pagebackref=true,breaklinks=true,letterpaper=true,colorlinks,bookmarks=false]{hyperref}
\usepackage[nameinlink, capitalise]{cleveref}
\crefformat{section}{#2section~#1#3}
\Crefformat{section}{#2Section~#1#3}

\theoremstyle{definition}

\newtheorem{theorem}{Theorem}

\begin{document}

\newpage
\begin{appendices}
\appendix
\setlength{\parskip}{0.5em}
% \crefalias{section}{appsec}
% We include dataset descriptions, experimental details, supplementary experiments, stability analysis, and running time analysis here.
In this supplement, we provide details of the datasets tested in the manuscript, and formally prove the renormalization's effect of compressing eigenvalue ranges.

\section{Dataset Details} \label{app:datasets}
\noindent\textbf{Citation networks.} Citation networks record documents' citation relationship \cite{sen2008collective}. In citation networks, vertices are documents and edges are citation links. A pair of vertices are connected by an undirected edge if and only if one cites the other. Each vertex is associated with a feature vector, which represents the document content. Feature vectors of Cora and CiteSeer are 0/1 vectors that have the same length as the dictionary size and indicate whether a word appears in a document. In PubMed and Large Cora, the feature vectors are the tf-idf weighted word vectors.

Cora and CiteSeer datasets are preprocessed and provided originlly by \cite{lu2003link, sen2008collective}. PubMed dataset first appears in \cite{namata2012query}. LargeCora is constructed by our own from Andrew McCallum's Cora Project. Andrew McCallum's Cora Project organized dozens of thousands of research papers into a topic hierarchy with 73 leaves. After removing the papers that belong to no topic and the ones that have no authors or title, a subset of 11881 papers is obtained. The task is to classify them into 10 highest-level topics in the topic hierarchy.
% In order to distinguish this dataset from the “Cora” dataset with 2708 papers as in \cite{kipf2016semi, yang2016revisiting, sen2008collective}, we name the dataset we constructed as “Large Cora”.

\noindent\textbf{Never Ending Language Learning (NELL).} NELL is a knowledge graph introduced by \cite{carlson2010toward}. \cite{yang2016revisiting} extracted an entity classification dataset from NELL and converted the knowledge graph into a single relation graph as follows. For each relation type $r$ in the knowledge graph, they created two new relation vertices $r_1$ and $r_2$ in the graph. For each triplet $(e_1, r, e_2)$ in the knowledge graph ($e_1$ and $e_2$ are any two entity vertices connected by the relation $r$), they created two edges $(e_1, r_1)$ and $(e_2, r_2)$. We follow \cite{kipf2016semi} to extend the data features by assigning a unique one-hot representation for every relation vertex.
% Finally, each vertex in the newly constructed graph is associated with a 61,278-dimensional sparse feature vector.\\

\noindent\textbf{ImageNet.} ImageNet \cite{russakovsky2015imagenet} is an image database organized according to the WordNet hierarchy. All categories of ImageNet form a graph through ``is a kind of'' relation. For example, drawbridge is a kind of bridge; bridge is a kind of construction; construction is a kind of artifact. According to \cite{wang2018zero}, the word embeddings of each category is learned from Wikipedia via GloVe text model \cite{pennington2014glove}. The AWA2 dataset \cite{xian2018zero} used in the experiment of zero-shot image recognition in the manuscript is a subset of ImageNet.

\section{Renormalization Trick} \label{app:self-loops}
In section 4.1, we revisited GCN model and gave a conclusion that the renormalization trick decreases the range of eigenvalues of Laplacian at least by factor $\frac{d_m}{d_m+1}$. Here we formally describe and prove this theoretical guarantee.

Given a positively weighted undirected graph with adjacency matrix $A$, its (symmetrically normalized) Laplacian is defined as $L_s=D^{-\frac12}(D-A)D^{-\frac12}$, where $D=\text{diag}(d_i)$ is degree matrix. The renormalization trick adds a self-loop to each vertex, so the renormalized adjacency matrix is defined as $\tilde{A}=A+I$. Corresponding degree matrix is $\tilde{D}=D+I$, and Laplacian is $\tilde{L}_s=\tilde{D}^{-\frac12}(\tilde{D}-\tilde{A})\tilde{D}^{-\frac12}$. We have following theorem.
\begin{theorem}\label{theorem:renorm}
    If the largest eigenvalue of $L_s$ is $\lambda_m$, then the largest eigenvalue of $\tilde{L_s}$ is no more than $\frac{d_m}{d_m+1}\lambda_m$, where $d_m=\max d_i$ is the graph degree (the largest degree of vertices).
\end{theorem}
\begin{proof}
    According to the property of eigenvalue,
    \begin{align}
        \tilde{\lambda}_m &= \max_{x} \frac{x^\top \tilde{L}_s x}{x^\top x} \\
        &= \max_{x} \frac{x^\top(D+I)^{-\frac12}D^{\frac12} L_s D^{\frac12}(D+I)^{-\frac12}x}{x^\top x} \nonumber
    \end{align}
    Let $y=D^{\frac12}(D+I)^{-\frac12}x$, then
    \begin{align}
        \tilde{\lambda}_m
        &= \max_{y} \frac{y\top L_s y}{y^\top(D+I)D^{-1}y}
        = \max_{y} \frac{y\top L_s y}{\sum_i{\frac{d_i+1}{d_i} y_i^2}} \nonumber\\
        &\le \max_{y} \frac{y\top L_s y}{\frac{d_m+1}{d_m} \sum_i{y_i^2}} \\
        &= \frac{d_m}{d_m+1} \max_{y} \frac{y\top L_s y}{y^\top y}
        = \frac{d_m}{d_m+1} \lambda_m \nonumber
        % &= \max_{y} \frac{y\top L_s y}{y^\top y} \cdot \frac{y^\top y}{y^\top(D+I)D^{-1}y} \\
        % &\le \max_{y} \frac{y\top L_s y}{y^\top y} \cdot \max_{y} \frac{y^\top y}{y^\top(D+I)D^{-1}y}
        % = \lambda_m
    \end{align}
\end{proof}
In conclusion, renormalization trick shrinks the range of eigenvalues of Laplacian from $[0, \lambda]$ to $[0, \frac{d_m}{d_m+1} \lambda_m]$. When all vertex degree $d_i$ are equal, the equality holds, so this upper bound for eigenvalues of renormalized Laplacian is tight.

\noindent\textbf{A Tighter Bound}
If we only have knowledge of graph's degree and largest eigenvalue of original Laplacian, above theorem is actually the best upper bound we could obtain. However, a stronger theorem can be proved if we know graph component structure. Consider a graph with $k$ connected components. Its adjacent matrix $A$, degree matrix $D$, Laplacian $L_s$, and their renormalized version $\tilde{A}, \tilde{D}, \tilde{L}_s$ are all block diagonal matrix. Each block is corresponding to a connected component.
\begin{align*}
    A=\begin{bmatrix}
        A^{(1)} && \\
        & \ddots   \\
        && A^{(k)}
    \end{bmatrix} & \quad
    \tilde{A}=\begin{bmatrix}
        \tilde{A}^{(1)} && \\
        & \ddots   \\
        && \tilde{A}^{(k)}
    \end{bmatrix} \\
    D=\begin{bmatrix}
        D^{(1)} && \\
        & \ddots   \\
        && D^{(k)}
    \end{bmatrix} & \quad
    \tilde{D}=\begin{bmatrix}
        \tilde{D}^{(1)} && \\
        & \ddots   \\
        && \tilde{D}^{(k)}
    \end{bmatrix} \\
    L_s=\begin{bmatrix}
        L_s^{(1)} && \\
        & \ddots   \\
        && L_s^{(k)}
    \end{bmatrix} & \quad
    \tilde{L}_s=\begin{bmatrix}
        \tilde{L}_s^{(1)} && \\
        & \ddots   \\
        && \tilde{L}_s^{(k)}
    \end{bmatrix}
\end{align*}
According to Theorem \ref{theorem:renorm}, if the largest eigenvalue of $L_s^{(k)}$ is $\lambda_m^{(k)}$, then the largest eigenvalue $\tilde{\lambda}^{(k)}_m$ of renormalized $\tilde{L}_s^{(k)}$ satisfies
\begin{equation}
    \tilde{\lambda}^{(k)}_m \le \frac{d^{(k)}_m}{d^{(k)}_m+1}\lambda_m^{(k)}.
\end{equation}
 As a result, the largest eigenvalue of the renormalized Laplacian of whole graph
\begin{align}
    \tilde{\lambda}_m = \max_k\{\tilde{\lambda}^{(k)}_m\}
    & \le \max_k\{\frac{d^{(k)}_m}{d^{(k)}_m+1}\lambda_m^{(k)}\} \label{eq:bound2}\\
    & \le \frac{d_m}{d_m+1}\lambda_m \label{eq:tighter}
\end{align}
The second inequality follows the fact of $d^{(k)}_m\le d_m$ and $\lambda_m^{(k)} \le \lambda_m$. Finally, we find another upper bound by analyzing renormalization trick's effect on each connected component. Eq. \ref{eq:tighter} indicates this new upper bound (eq. \ref{eq:bound2}) is tighter than Theorem \ref{theorem:renorm}.

\end{appendices}

% \bibliography{parw}
% \bibliographystyle{plainnat}

{\small
\bibliographystyle{ieee}
\bibliography{parw}
}
\end{document}
